# Supplementary material for: Ising distribution as a latent variable model
Source: arXiv:1803.02598 ancillary file (2019-05-10)
Supplement: Supplementary file 1 [file wohrer_supplementary.pdf]

# SUPPLEMENTARY MATERIAL

**The Ising distribution as a latent variable model**

Adrien Wohrer*

*Université Clermont Auvergne, CNRS, SIGMA Clermont,*

*Institut Pascal, F-63000 Clermont-Ferrand, France.*

## Abstract

In this supplementary document, I provide additional figures and mathematical details, supporting some of the statements made in the main text.

**Section 1:** details two ways of predicting the Ising spin covariance matrix $\mathbf{C}$, based on the variational Cox approximation. In all of my numerical tests, these two predictions provided very similar results. Furthermore, the amount of deviation between the two predictions was predictive of the global success of the approximation.

**Section 2:** shows the fit performance of a modified variational Cox approximation, using zero diagonal couplings $J_{ii}$. This largely suppresses the bias observed in the main text, and the resulting approximation ends up very close to the adaptive TAP approximation in all tested conditions.

**Section 3:** expands on the chosen generative model for $\mathbf{J}$ (eq. (32) from the main text), proving that the SK model is indeed recovered when $\kappa \to +\infty$.

**Section 4:** works through the approximate formulas for the moments of the Cox distribution (Appendix E from the main text), that I used to speed up computations.

* adrien.wohrer@uca.fr

## I. COHERENCE OF MOMENT PREDICTIONS IN THE COX APPROXIMATION

*Reminder from the main text*

If a given Ising distribution $P(\mathbf{s})$ has spin moments $(\mathbf{m}, \mathbf{C})$, then the corresponding moments of the latent field distribution $P(\mathbf{r})$ are

$$\boldsymbol{\mu} = \mathbf{h} + \mathbf{J}\mathbf{m}, \tag{1}$$

$$\boldsymbol{\Sigma} = \mathbf{J} + \mathbf{J}\mathbf{C}\mathbf{J}. \tag{2}$$

Given some Cox distribution $Q$ of parameters $(\boldsymbol{\mu}, \boldsymbol{\Sigma})$, eq. (1)-(2) provide a natural reparametrization in function of the 'equivalent Ising spin moments' $(\mathbf{m}, \mathbf{C})$.

In the variational Cox approximation, parameters $(\boldsymbol{\mu}, \boldsymbol{\Sigma})$ are chosen as stationary points of the reversed KL divergence between $Q(\mathbf{r})$ and $P(\mathbf{r})$. In terms of the reparametrization variables $(\mathbf{m}, \mathbf{C})$, this leads to the equations

$$m_i = \int_{x\in\mathbb{R}} \tanh\left(\mu_i + x\sqrt{\Sigma_{ii}}\right) \phi(x)\mathrm{d}x, \tag{3}$$

$$(\mathbf{C}^{-1})_{ij} = \left[\int_{x\in\mathbb{R}} \left(1 - \tanh^2\left(\mu_i + x\sqrt{\Sigma_{ii}}\right)\right) \phi(x)\mathrm{d}x\right]^{-1} \delta_{ij} - J_{ij} \tag{4}$$

Together, eq. (1)-(4) characterize the 'variational Cox' approximation from the main text. The corresponding values of $(\mathbf{m}, \mathbf{C})$ constitute approximations of the Ising spin moments.

However, given the approximating Cox distribution $Q(\boldsymbol{\mu}, \boldsymbol{\Sigma})$, another natural prediction for the Ising spin moments would be the resulting spin moments for distribution $Q$, which write

$$\mathrm{E}_Q(s_i) = \int_{x\in\mathbb{R}} \tanh\left(\mu_i + x\sqrt{\Sigma_{ii}}\right) \phi(x)\mathrm{d}x, \tag{5}$$

$$\mathrm{Cov}_Q(s_i, s_j) = \int_{(x,y)\in\mathbb{R}^2} \tanh\left(\mu_i + x\sqrt{\Sigma_{ii}}\right) \tanh\left(\mu_j + y\sqrt{\Sigma_{jj}}\right) \left[\phi_2(x, y|\rho_{ij}) - \phi(x)\phi(y)\right]\mathrm{d}x\mathrm{d}y, \tag{6}$$

with $\rho_{ij} = \Sigma_{ij}/\sqrt{\Sigma_{ii}\Sigma_{jj}}$, $\phi$ the standard normal density, and $\phi_2(\cdot|\rho)$ the standard bivariate normal density with correlation $\rho$.

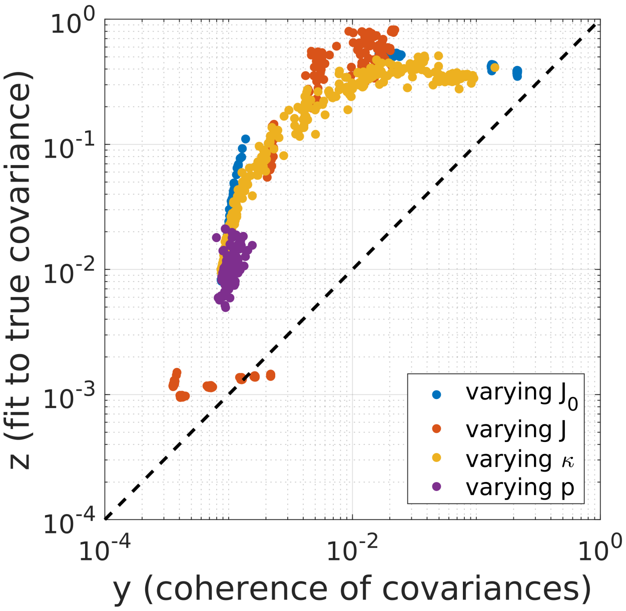


FIG. 1. Coherence of predictions for the covariance matrix in the Cox approximation. Each dot represents a configuration $(\mathbf{h}, \mathbf{J})$ from the numerical tests of the main text, with different colors indicating the generative parameter being varied. The abscissa is the self-coherence of covariance predictions $y$ (eq. (7)) for the variational Cox approximation on this configuration. The ordinate is the fit value $z$ (eq. (8)) of the variational Cox approximation on this configuration.

*Coherence of covariance predictions*

In the variational Cox approximation, the predicted magnetizations are always coherent : the values $m_i$ at the stationary point (eq. (3)) correspond exactly to the first moments of the corresponding Cox distribution $Q$ (eq. (5)).

The same does not hold for predicted covariances : matrix $\mathbf{C}$, as given by eq. (4), is formally very different from the spin covariance in the resulting Cox distribution, eq. (6). However, if $Q$ is a good approximation of $P$, we expect both predictions of $\mathbf{C}$ to be very close. To check this, once the variational Cox solution has been found, I compute the following divergence between the two predictions for the covariance matrix :

$$y = \frac{1}{N^2} \sum_{i,j} \left| C_{ij} - \mathrm{Cov}_Q(s_j, s_j) \right|, \tag{7}$$

and compare it to the approximation's fit value on the true Ising moments :

$$z = \frac{1}{N^2} \sum_{i,j} \left| C_{ij} - C^\star_{ij} \right|. \tag{8}$$

Figure 1 displays these two quantities, at the solution of the variational Cox approximation, for every configuration of $(\mathbf{h}, \mathbf{J})$ that I tested numerically (see Section 'Numerical Tests' from the main text). It reveals that $y$ is, on average, an order of magnitude smaller than $z$. This means that choosing either eq. (4) or eq. (6) as the effective covariance prediction will have a minimal impact on the fit value with respect to true covariance $\mathbf{C}^\star$. Whichever prediction is chosen, a good fit value $z$ simply indicates that the latent field $P(\mathbf{r})$ is close to being normally distributed.

Note that, in practical applications, the true moments are unknown, and so is the fit value $z$. However, the coherence measure $y$ can actually be computed. If this number is large, it very likely indicates that the variational Cox method has failed to target the true moments of the distribution, because parameters $(\mathbf{h}, \mathbf{J})$ are not in the 'mean field domain'.

## II. VARIATIONAL COX APPROXIMATION WITH ZERO DIAGONAL

In this section, I present the fit performance of the variational Cox approximation, eq. (1)-(4), when matrix $\mathbf{J}$ is given a *zero diagonal*. In this case, $\mathbf{J}$ is not definite positive, and the Ising latent field distribution $P(\mathbf{r})$ is not properly defined. However, the fixed point equation (1)-(4) generally retains a well-defined solution (except in a few tested configurations far inside the ferromagnetic or spin glass phases).

Figure 2 shows that the resulting approximation has a fit performance extremely similar to the adaptive TAP solution from the main text. This is one of the arguments suggesting that the main source of bias of the variational Cox approximation compared to the adaptive TAP approximation is the presence of nonzero diagonal terms $J_{ii}$.

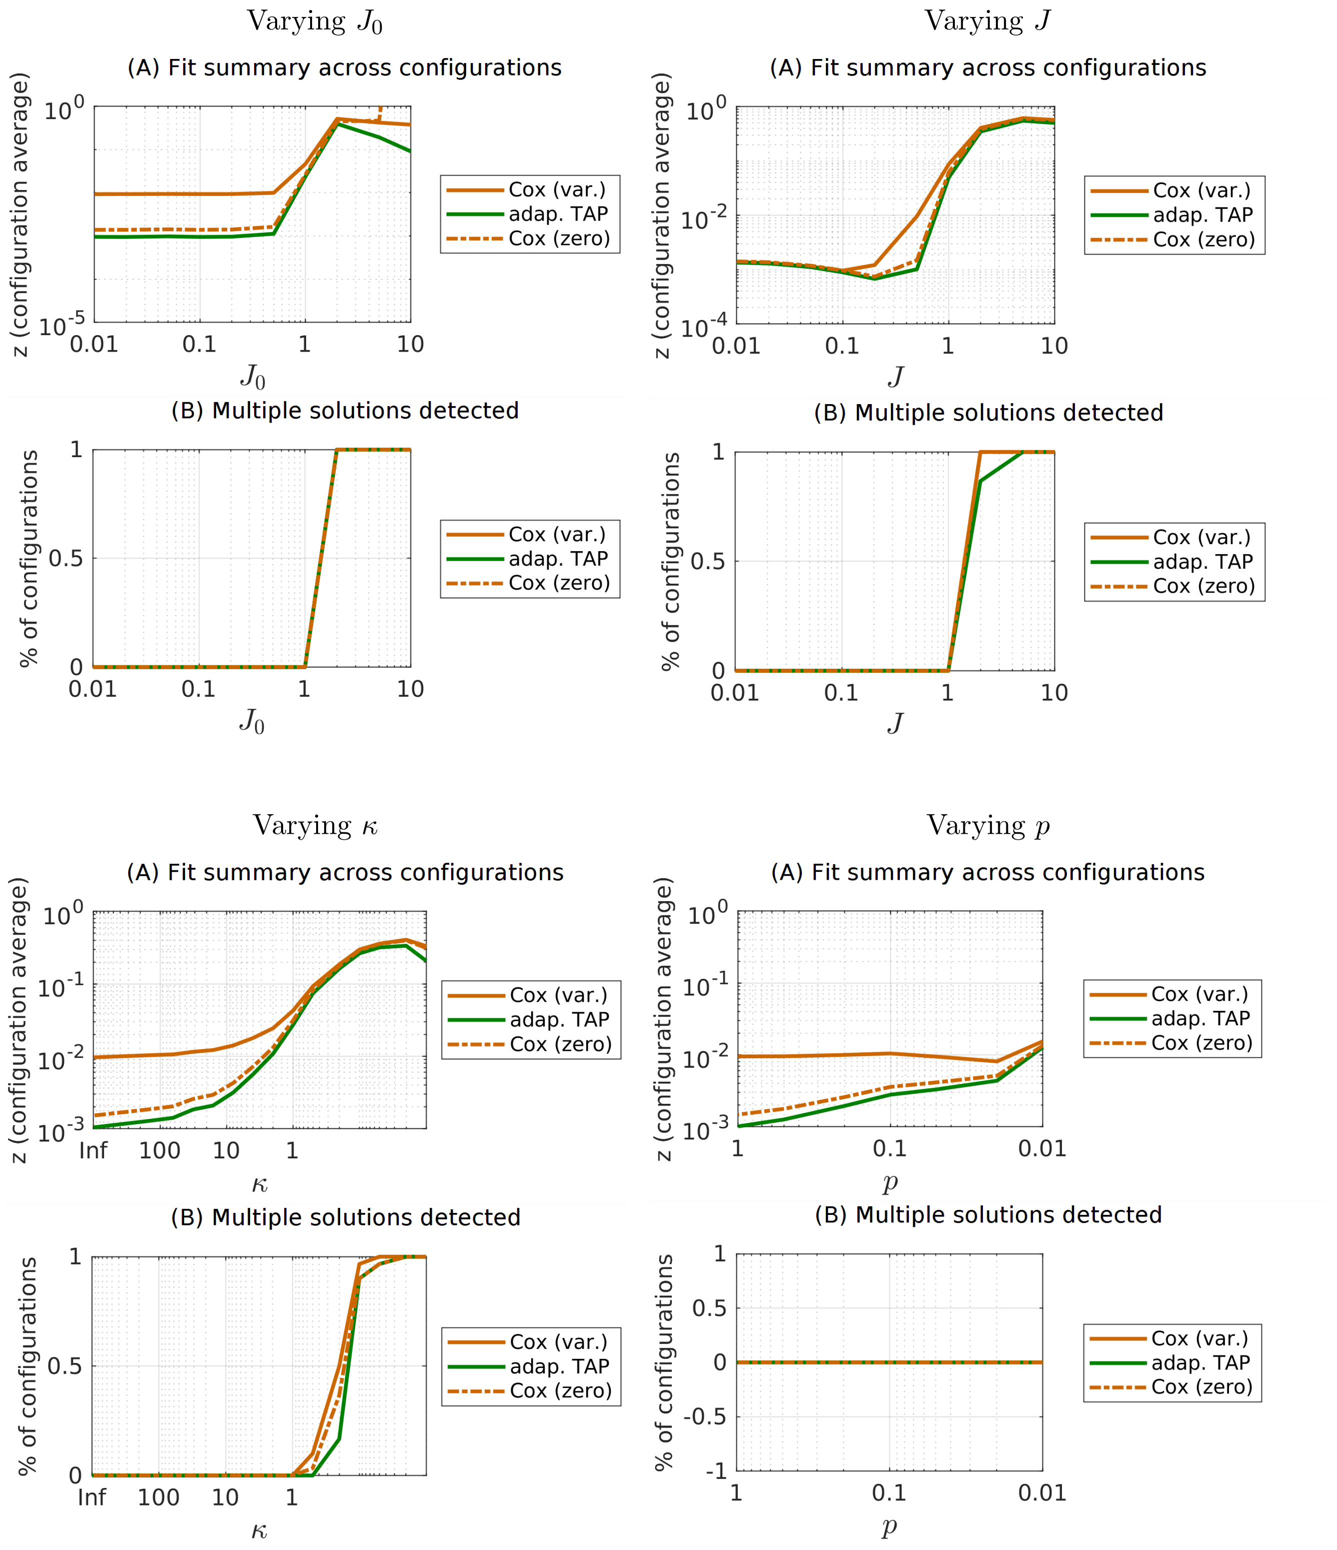


FIG. 2. Variational Cox approximation with zero self-couplings $J_{ii}$, tested on the same matrices $\mathbf{J}$ as in Figures 2-6 from the main text. The variational Cox approximation from the main text (with nonzero $J_{ii}$) and adaptive TAP approximation are redrawn for comparison.

## III. LINK BETWEEN THE SK AND WISHART MODELS FOR J

In the main text, I introduce the following distribution for $\mathbf{J}$ :

$$\mathbf{J} = \frac{J_0}{N}\mathbf{1} + \frac{J}{\sqrt{\kappa N}}\mathbf{X}_\kappa \mathbf{X}_\kappa^\top \tag{9}$$

with $\mathbf{X}_\kappa$ an $N \times \kappa N$ matrix of independent standard normal entries (i.e., each $X_{ij} \sim \mathcal{N}(0,1)$ independently from the others). In statistics, the probabilistic distribution for matrix $\mathbf{X}_\kappa \mathbf{X}_\kappa^\top$ is known as the *Wishart distribution.* Then, I claim without much explanation that the SK model is recovered when $\kappa \to +\infty$. Here, I clarify this claim.

Let us note, for lighter argumentation, $K = \kappa N$ and introduce the random matrix

$$\mathbf{W} = K^{-1/2}\mathbf{X}_K \mathbf{X}_K^\top,$$

$\mathbf{X}_K$ being the same matrix as above (of size $N \times K$). Then, our precise statement is the following :

**Proposition 1.** *When $K \to +\infty$, the upper-diagonal part of $\mathbf{W}$ converges in law to a set of $N(N-1)/2$ independent standard normal variables.*

Going back to definition (9), one can check that this implies exactly the SK distribution for the off-diagonal elements of matrix $\mathbf{J}$ when $\kappa \to +\infty$, i.e., the off-diagonal elements $J_{ij}$ become independently distributed following $\mathcal{N}(J_0/N, J/N)$.

The proof of Prop. 1 can be found in classic references on the Wishart distribution, but for the sake of completeness I sketch it here. Consider the moment generating function (m.g.f.) of matrix $\mathbf{W}$, defined as $F(\mathbf{Z}) := \mathrm{E}\left[\exp\left(\sum_{i\leq j} Z_{ij}W_{ij}\right)\right]$, where $\mathbf{Z}$ is an upper-triangular matrix of dummy variables associated to the $N(N+1)/2$ random variables $\{W_{ij}\}_{i\leq j}$ and the expectation is with respect to the distribution of $\mathbf{W}$. The m.g.f. of the Wishart distribution is well-known. Reexpressed for matrix $\mathbf{W}$, it writes

$$F(\mathbf{Z}) = \det\left(\mathbf{I} - 2K^{-1/2}\overline{\mathbf{Z}}\right)^{-K/2},$$

with $\overline{\mathbf{Z}} = (\mathbf{Z} + \mathbf{Z}^\top)/2$ and $\mathbf{I}$ the identity matrix.

Applying a classic expansion of the determinant (e.g., based on the fact that $\det(e^{\mathbf{A}}) = e^{\mathrm{Tr}(\mathbf{A})}$), for small $\epsilon$ one has

$$\log\det\left(\mathbf{I} + \epsilon\overline{\mathbf{Z}}\right) = \epsilon\,\mathrm{Tr}(\overline{\mathbf{Z}}) - \frac{\epsilon^2}{2}\,\mathrm{Tr}(\overline{\mathbf{Z}}^2) + o(\epsilon^2)$$

and thus, we obtain

$$\log F(\mathbf{Z}) = \sum_i \left(K^{1/2} Z_{ii} + Z_{ii}^2\right) + \frac{1}{2}\sum_{i<j} Z_{ij}^2 + o(1) \qquad (K \to +\infty).$$

Thus, in the limit $K \to +\infty$, the m.g.f. factorizes over the dummy variables $Z_{ij}$, which implies that the corresponding random variables $W_{ij}$ become independent. Furthermore, the m.g.f. for an off-diagonal element $W_{ij}$ writes

$$F_{W_{ij}}(Z_{ij}) = e^{Z_{ij}^2/2}$$

where we recognize the m.g.f. of a standard normal random variable.

## IV. APPROXIMATE FORMULAS FOR THE COX MOMENTS

### IV.1. Rationale of the approximation

The moments of the Cox distribution $Q(\boldsymbol{\mu}, \boldsymbol{\Sigma})$ are exactly given as $(i \neq j)$ :

$$m_i = \int_{x\in\mathbb{R}} \tanh\left(\mu_i + x\sqrt{\Sigma_{ii}}\right) \phi(x)\mathrm{d}x \tag{10}$$

$$C_{ij} = \int_{(x,y)\in\mathbb{R}^2} \tanh\left(\mu_i + x\sqrt{\Sigma_{ii}}\right) \tanh\left(\mu_j + y\sqrt{\Sigma_{jj}}\right) \left[\phi_2(x,y|\rho_{ij}) - \phi(x)\phi(y)\right]\mathrm{d}x\mathrm{d}y. \tag{11}$$

Besides, the variational Cox approximation also relies on two other quantities of similar nature (see main text) :

$$F_i = \int_{x\in\mathbb{R}} \log 2\cosh\left(\mu_i + x\sqrt{\Sigma_{ii}}\right) \phi(x)\mathrm{d}x$$

$$d_i = 1 - \int_{x\in\mathbb{R}} \tanh^2\left(\mu_i + x\sqrt{\Sigma_{ii}}\right) \phi(x)\mathrm{d}x$$

Number $F_i$ is required to estimate the variational free energy (eq. 13 from the main text), and number $d_i$ is involved in the equation defining stationary points of this free energy (eq. 17 from the main text).

All these quantities can be easily estimated by numerical integration (for example, Simpson quadrature), but the overall computation time quickly becomes forbidding, as these estimations must be done for each pair of spins, and on many iterations to target the fixed point. I found it more convenient to use approximate formulas, based on approximating the logistic function

$$L(r) := \frac{1}{1+e^{-2r}}$$

by the following sum of Gaussian functions :

$$L^{\mathrm{app}}(r) = \Phi\left(\frac{r}{\kappa}\right) + \nu\phi'\left(\frac{r}{\lambda}\right), \tag{12}$$

with $\phi(x) = 1/\sqrt{2\pi}\exp(-x^2/2)$ the standard normal distribution, $\Phi(x) := \int_{-\infty}^{x}\phi(u)\mathrm{d}u$ the standard normal cumulative distribution, and $\phi'(r) = -r\phi(r)$.

For well-chosen parameters $(\kappa, \nu, \lambda) \simeq (0.7072, 0.1648, 0.9712)$, one has $L(x) = L^{\mathrm{app}}(x) + \epsilon(x)$ and $\|\epsilon\|_\infty < 0.001$ on the whole real line. The approximation also applies to the primitive, with $\|\int_0^x \epsilon\|_\infty < 0.001$, and to the first derivative, with $\|\epsilon'\|_\infty < 0.0033$.

As the convolution product of two Gaussian functions remains Gaussian, this replacement allows to compute analytically all the formulas. Below, I detail this computation for $m_i$ and $C_{ij}$ (the formulas for $F_i$ and $d_i$ being derived in a very similar fashion).

Before presenting the actual formulas, we can already discuss their accuracy. Let $m_i^{\text{app}}$ and $C_{ij}^{\text{app}}$ denote the formulas equivalent to eq. (10)-(11) but using function $\tanh^{\text{app}}(r) = 2L^{\text{app}}(r) - 1$. Writing $\tanh(r) = \tanh^{\text{app}}(r) + 2\epsilon(r)$ in eq. (10)-(11), and applying standard majorations using the facts that $\|\tanh\|_\infty = 1$, $\int_x \phi(x)\mathrm{d}x = 1$ and $\int_{x,y} \phi_2(x, y|\rho)\mathrm{d}x\mathrm{d}y = 1$, we find that

$$
\begin{aligned}
|m_i - m_i^{\text{app}}| &\leq 2\|\epsilon\|_\infty & &< 0.002 \\
|C_{ij} - C_{ij}^{\text{app}}| &\leq 8\|\epsilon\|_\infty + 8\|\epsilon\|_\infty^2 & &< 0.008
\end{aligned}
$$

so we expect maximum errors in the order of $10^{-3}$, and generally much less.

In my tests, the approximation errors were always small enough to yield no noticeable difference in the final solution of the Cox fixed point equations, whether we used the approximation or a lengthier Simpson quadrature. At the same time, computation times were cut by some two orders of magnitude.

### IV.2. Notations and reformulation

For the purpose of the following derivations, I adopt a slightly different formulation of eq. (10)-(11), which leads to simpler formulas. Let us note, in any dimension, $\mathcal{N}(\mathbf{x}|\mathbf{A})$ the centered normal distribution of (co)variance $\mathbf{A}$, that is :

$$\mathcal{N}(\mathbf{x}|\mathbf{A}) := |2\pi\mathbf{A}|^{-1/2} \exp\left(-\frac{1}{2}\mathbf{x}^\top \mathbf{A}^{-1}\mathbf{x}\right).$$

In eq. (10)-(11), the standard normal distribution corresponds to $\phi(x) = \mathcal{N}(x|1)$, whereas the standard bivariate normal distribution $\phi_2(x, y|\rho)$ can be defined in either of two forms :

$$\phi_2(x, y|\rho) = \mathcal{N}\left(\begin{pmatrix} x \\ y \end{pmatrix} \middle| \begin{pmatrix} 1 & \rho \\ \rho & 1 \end{pmatrix}\right) \tag{13}$$

$$= \mathcal{N}(x|1)\mathcal{N}(y - \rho x|1 - \rho^2). \tag{14}$$

The approximation for $L$, eq. (12), can then be rewritten as

$$L^{\text{app}}(r) = \Phi\left(\frac{r}{\kappa}\right) - \nu r \mathcal{N}(r|\lambda^2) \tag{15}$$

With these notations settled, we introduce the two following functions :

$$f_1(a,b) := \int_{u\in\mathbb{R}} L(u)\mathcal{N}(u-b|a^2)\mathrm{d}u, \tag{16}$$

$$f_2(a,b,c,d,\rho) := \int_{u,v} L(u)L(v)\mathcal{N}\left(\begin{pmatrix}u\\v\end{pmatrix} - \begin{pmatrix}b\\d\end{pmatrix}\middle|\begin{pmatrix}a^2 & \rho ac\\ \rho ac & c^2\end{pmatrix}\right)\mathrm{d}u\mathrm{d}v, \tag{17}$$

Then, one checks easily that the moments of the Cox distribution $Q(\boldsymbol{\mu},\boldsymbol{\Sigma})$, eq. (10)-(11), can be reexpressed as

$$\begin{aligned}
m_i &= 2f_1\big(\sqrt{\Sigma_{ii}},\mu_i\big) - 1,\\
C_{ij} &= 4f_2\big(\sqrt{\Sigma_{ii}},\mu_i,\sqrt{\Sigma_{jj}},\mu_j,\rho_{ij}\big) - 4f_1\big(\sqrt{\Sigma_{ii}},\mu_i\big)f_1\big(\sqrt{\Sigma_{jj}},\mu_j\big),
\end{aligned}$$

with $\rho_{ij} := \Sigma_{ij}/\sqrt{\Sigma_{ii}\Sigma_{jj}}$.

Replacing $L$ by its approximation $L^{\text{app}}$, we can build approximations for $f_1$ and $f_2$ that will yield the approximate moments $m_i^{\text{app}}$ and $C_{ij}^{\text{app}}$.

### IV.3. Basic convolution result

In the sequel, we will make repeated use of the following relation :

$$\mathcal{N}(\mathbf{x}-\mathbf{b}|\mathbf{A}_1)\mathcal{N}(\mathbf{x}|\mathbf{A}_2) = \mathcal{N}(\mathbf{b}|\mathbf{A}_1+\mathbf{A}_2)\mathcal{N}(\mathbf{x}-\boldsymbol{\beta}|\mathbf{M}) \tag{18}$$

with $\mathbf{M} := [\mathbf{A}_1^{-1}+\mathbf{A}_2^{-1}]^{-1}$ and $\boldsymbol{\beta} = \mathbf{A}_2(\mathbf{A}_1+\mathbf{A}_2)^{-1}\mathbf{b}$. Integrated over $\mathbf{x}$, it implies that the convolution product of $\mathcal{N}(\mathbf{A}_1)$ and $\mathcal{N}(\mathbf{A}_2)$ is $\mathcal{N}(\mathbf{A}_1+\mathbf{A}_2)$, a famous result if ever. In particular, it implies the following convolution result, that we will use repeatedly :

$$\begin{aligned}
\int_u \mathcal{N}(u-b|a^2)\Phi\left(\frac{u-d}{c}\right)\mathrm{d}u &= \int_u\int_{s>0}\mathcal{N}(u-b|a^2)\mathcal{N}(u-d-s|c^2)\mathrm{d}u\mathrm{d}s\\
&= \int_{s>0}\mathcal{N}(b-d-s|a^2+c^2)\mathrm{d}s \qquad \text{(convolution in } u\text{)}\\
&= \Phi\left(\frac{b-d}{\sqrt{a^2+c^2}}\right) \qquad (19)
\end{aligned}$$

### IV.4. Approximation for $m_i$

With the previous results, the approximation for $f_1$ writes

$$
\begin{aligned}
f_1^{\text{app}}(a,b) &:= \int_u L^{\text{app}}(u)\mathcal{N}(u-b|a^2)\mathrm{d}u \\
&= \int_u \Phi(u/\kappa)\mathcal{N}(u-b|a^2)\mathrm{d}u - \nu \int_u u\mathcal{N}(u|\lambda^2)\mathcal{N}(u-b|a^2)\mathrm{d}u \\
&= \Phi\left(\frac{b}{\sqrt{\kappa^2+a^2}}\right) - \nu\mathcal{N}(b|\lambda^2+a^2)\frac{\lambda^2}{a^2+\lambda^2}b
\end{aligned}
$$

after an application of (19) and (18), and an integration in $u$.

As in the main text, we can introduce the rescaled parameters

$$
\begin{aligned}
x_i &:= \frac{\mu_i}{\sqrt{\Sigma_{ii}}} \\
k_i &:= \frac{\sqrt{\Sigma_{ii}}}{\sqrt{\kappa^2+\Sigma_{ii}}} \\
l_i &:= \frac{\sqrt{\Sigma_{ii}}}{\sqrt{\lambda^2+\Sigma_{ii}}}
\end{aligned}
$$

and rewrite $m_i^{\text{app}} = 2f_1^{\text{app}}(\sqrt{\Sigma_{ii}}, \mu_i) - 1$ as

$$
m_i^{\text{app}} = 2\left[\Phi\left(x_i k_i\right) + \nu(1-l_i^2)\phi'\left(x_i l_i\right)\right] - 1 \tag{20}
$$

### IV.5. Approximation for $C_{ij}$

I now turn to the approximation of $f_2$ in eq. (17). We introduce matrix $\mathbf{A} = \begin{pmatrix} a^2 & \rho ac \\ \rho ac & c^2 \end{pmatrix}$, and split $f_2^{\text{app}}$ in 4 terms :

$$
\begin{aligned}
f_2^{\text{app}}(a,b,c,d,\rho) &:= \int_u\int_v L^{\text{app}}(u)L^{\text{app}}(v)\mathcal{N}\left(\begin{pmatrix} u \\ v\end{pmatrix} - \begin{pmatrix} b \\ d\end{pmatrix}\middle| \mathbf{A}\right)\mathrm{d}u\mathrm{d}v \\
&= T_0 - \nu T_1 - \nu T_1^{[\text{sym}]} + \nu^2 T_2
\end{aligned}
$$

with the three types of terms derived below.

*Term $T_0$*

It is derived as

$$\begin{aligned}
T_0 &= \int_u \int_v \Phi(u/\kappa)\Phi(v/\kappa)\mathcal{N}\left(\begin{pmatrix} u \\ v \end{pmatrix} - \begin{pmatrix} b \\ d \end{pmatrix} \middle| \mathbf{A}\right) \mathrm{d}u\mathrm{d}v \\
&= \int_{s>0}\int_{t>0}\int_u\int_v \mathcal{N}\left(\begin{pmatrix} u \\ v \end{pmatrix} - \begin{pmatrix} s \\ t \end{pmatrix} \middle| \kappa^2\mathbf{I}\right) \mathcal{N}\left(\begin{pmatrix} u \\ v \end{pmatrix} - \begin{pmatrix} b \\ d \end{pmatrix} \middle| \mathbf{A}\right) \mathrm{d}u\mathrm{d}v\mathrm{d}s\mathrm{d}t \\
&= \int_{s>0}\int_{t>0} \mathcal{N}\left(\begin{pmatrix} b \\ d \end{pmatrix} - \begin{pmatrix} s \\ t \end{pmatrix} \middle| \kappa^2\mathbf{I} + \mathbf{A}\right) \mathrm{d}s\mathrm{d}t \\
&= \Phi_2\left(\frac{b}{\sqrt{a^2+\kappa^2}}, \frac{d}{\sqrt{c^2+\kappa^2}} \middle| \frac{\rho ac}{\sqrt{(a^2+\kappa^2)(c^2+\kappa^2)}}\right)
\end{aligned}$$

where $\Phi_2(x,y|\rho) := \int_{(u,v)=(-\infty,-\infty)}^{x,y} \phi_2(u,v|\rho)\mathrm{d}u\mathrm{d}v$ is the standard bivariate cumulative distribution, for which efficient numerical routines are easily available.

*Term $T_1$*

It is derived as

$$\begin{aligned}
T_1 &= \int_u \int_v \Phi(u/\kappa) v\mathcal{N}(v|\lambda^2)\mathcal{N}\left(\begin{pmatrix} u \\ v \end{pmatrix} - \begin{pmatrix} b \\ d \end{pmatrix} \middle| \begin{pmatrix} a^2 & \rho ac \\ \rho ac & c^2 \end{pmatrix}\right) \mathrm{d}u\mathrm{d}v \\
&= \int_{s>0}\int_u\int_v \mathcal{N}(u-s|\kappa^2) v\mathcal{N}(v|\lambda^2)\mathcal{N}(v-d|c^2)\mathcal{N}(u-b-\rho(v-d)|a(1-\rho^2))\mathrm{d}s\mathrm{d}u\mathrm{d}v
\end{aligned}$$

using the integral representation of $\Phi$, and the representation of $\phi_2$ in eq. (14).

Integrating over $u$, then over $s$, and finally applying (18), we arrive at

$$T_1 = \mathcal{N}(d|\lambda^2 + c^2)\int_v v\mathcal{N}(v-\beta|m^2)\Phi\left(\frac{\rho v - \rho d + b}{\sqrt{a^2(1-\rho^2)+\kappa^2}}\right)\mathrm{d}v$$

with the following definitions :

$$m^2 := \frac{\lambda^2 c^2}{\lambda^2 + c^2} \quad , \quad \beta := \frac{\lambda^2}{\lambda^2 + c^2} d$$

The remaining integral can be performed using the fact that $v\mathcal{N}(v-\beta|m^2) = \beta\mathcal{N}(v-\beta|m^2) - m\mathcal{N}'(v-\beta|m^2)$, followed by an integration by parts and another application of (19). We obtain the final result

$$T_1 = \frac{\lambda^2}{\lambda^2+c^2}\mathcal{N}(d|\lambda^2+c^2)\left(d\Phi(\Delta/S) + \rho c^2\mathcal{N}(\Delta|S^2)\right)$$

with the following definitions :

$$\Delta := b - \rho\frac{c^2 d}{\lambda^2+c^2}$$
$$S^2 := a^2(1-\rho^2) + \kappa^2 + \rho^2\frac{\lambda^2 c^2}{\lambda^2+c^2}$$

The symmetric term $T_1^{[\mathrm{sym}]}$ is obtained by inverting the roles of $(a,b)$ and $(c,d)$.

*Term $T_2$*

It is derived as

$$\begin{aligned} T_2 &= \int_u\int_v uv\mathcal{N}(u|\lambda^2)\mathcal{N}(v|\lambda^2)\mathcal{N}\left(\begin{pmatrix}u\\v\end{pmatrix} - \begin{pmatrix}b\\d\end{pmatrix}\middle|\mathbf{A}\right)\mathrm{d}u\mathrm{d}v \\ &= \mathcal{N}\left(\begin{pmatrix}b\\d\end{pmatrix}\middle|\lambda^2\mathbf{I}+\mathbf{A}\right)\int_u\int_v uv\mathcal{N}\left(\begin{pmatrix}u\\v\end{pmatrix} - \boldsymbol{\beta}\middle|\mathbf{M}\right)\mathrm{d}u\mathrm{d}v \qquad \text{(with (18))} \\ &= \mathcal{N}\left(\begin{pmatrix}b\\d\end{pmatrix}\middle|\lambda^2\mathbf{I}+\mathbf{A}\right)\left(\beta_1\beta_2 + M_{12}\right) \end{aligned}$$

for the following vector and matrix :

$$\mathbf{M}^{-1} = \lambda^{-2}\mathbf{I} + \begin{pmatrix}a^2 & \rho ac\\ \rho ac & c^2\end{pmatrix}^{-1} \quad , \quad \boldsymbol{\beta} = \lambda^2\left(\lambda^2\mathbf{I} + \begin{pmatrix}a^2 & \rho ac\\ \rho ac & c^2\end{pmatrix}\right)^{-1}\begin{pmatrix}b\\d\end{pmatrix}$$

The corresponding expressions for $\beta_1\beta_2$ and $M_{12}$ can be computed explicitly, as

$$M_{12} = \lambda^4\frac{Z}{XY-Z^2}$$
$$\beta_1\beta_2 = \lambda^4\frac{(bX-dZ)(dY-bZ)}{(XY-Z^2)^2}$$

with

$$X := c^2+\lambda^2 \quad , \quad Y := a^2+\lambda^2 \quad , \quad Z := \rho ac.$$

*Summary*

Collecting these results, using the same notations as above :

$$x_i := \frac{\mu_i}{\sqrt{\Sigma_{ii}}}$$
$$k_i := \frac{\sqrt{\Sigma_{ii}}}{\sqrt{\kappa^2 + \Sigma_{ii}}}$$
$$l_i := \frac{\sqrt{\Sigma_{ii}}}{\sqrt{\lambda^2 + \Sigma_{ii}}}$$

the intermediate quantities $\Delta$ and $S^2$ can be expressed as

$$\Delta_{ij} := \mu_j - \rho_{ij}\mu_i l_i^2,$$
$$S_{ij}^2 := \Sigma_{jj} + \kappa^2 + \rho_{ij}^2(\lambda^2 l_i^2 - \Sigma_{jj}),$$

Then, the approximated second moment $C_{ij}$ of the Cox distribution writes

$$C_{ij}^{\text{app}} = 4f_{ij}^{\text{app}} - (1 + m_i^{\text{app}})(1 + m_j^{\text{app}}) \tag{21}$$

with $m_i^{\text{app}}$ given by eq. (20), and (after some extra work on the $T_2$ term) :

$$\begin{aligned} f_{ij}^{\text{app}} =& \Phi_2\left(x_i k_i, x_j k_j \middle| \rho_{ij} k_i k_j\right) \\ &+ \nu(1 - l_i^2)\phi'\left(x_i l_i\right)\left[\mu_i \Phi\left(\frac{\Delta_{ij}}{S_{ij}}\right) + \frac{\rho_{ij}\Sigma_{ii}}{S_{ij}}\phi\left(\frac{\Delta_{ij}}{S_{ij}}\right)\right] \\ &+ \nu(1 - l_j^2)\phi'\left(x_j l_j\right)\left[\mu_j \Phi\left(\frac{\Delta_{ji}}{S_{ji}}\right) + \frac{\rho_{ij}\Sigma_{jj}}{S_{ji}}\phi\left(\frac{\Delta_{ji}}{S_{ji}}\right)\right] \\ &+ \nu^2 \frac{l_i^2(1 - l_i^2) l_j^2 (1 - l_j^2)}{(1 - \rho_{ij}^2 l_i^2 l_j^2)^2}\phi_2\left(x_i l_i, x_j l_j \middle| \rho_{ij} l_i l_j\right)\left[\Sigma_{ij}(1 - x_i^2 l_i^2 - x_j^2 l_j^2 - \rho_{ij}^2 l_i^2 l_j^2) + \mu_i\mu_j(1 + \rho_{ij}^2 l_i^2 l_j^2)\right] \end{aligned}$$
